# Supplementary material for: Periodic skyrmionic textures via conformal cartographic projections
Source: arXiv:2310.08964 source file (2024-06-23)

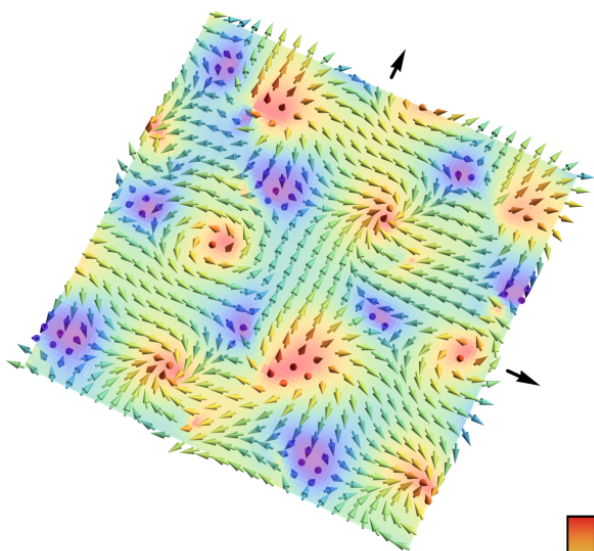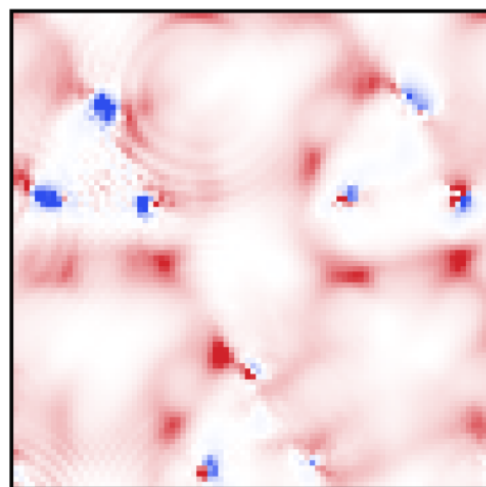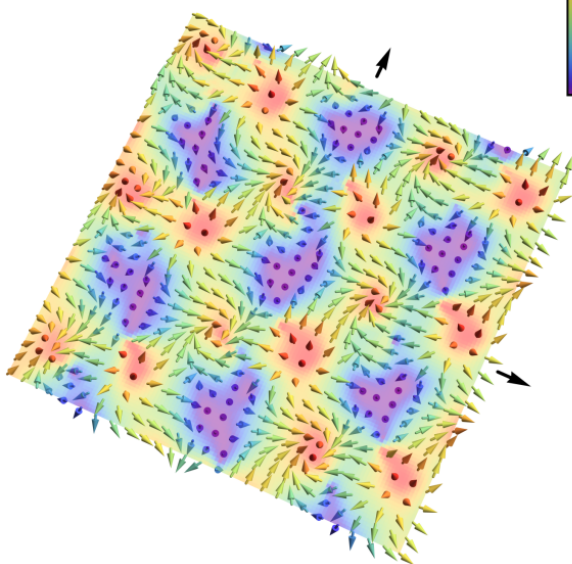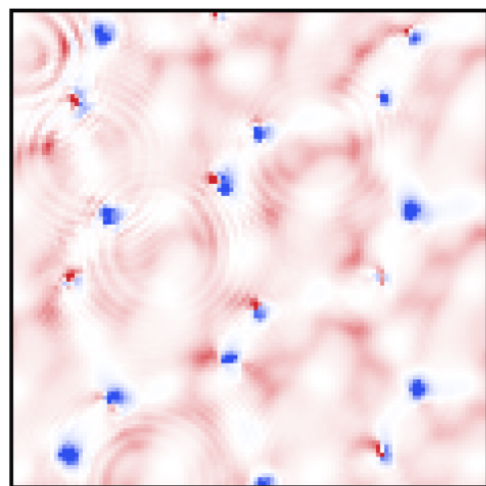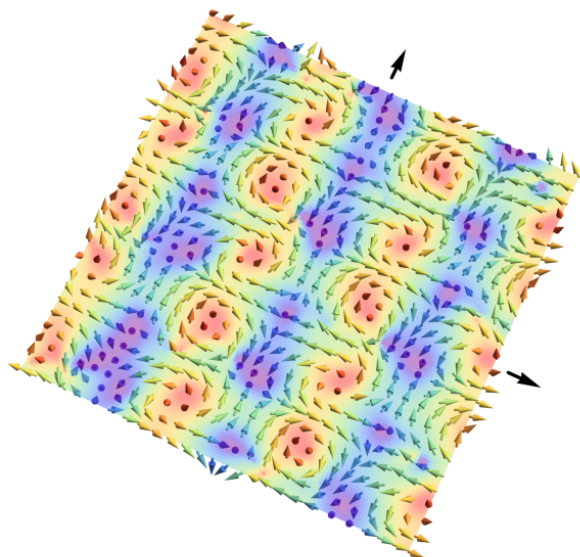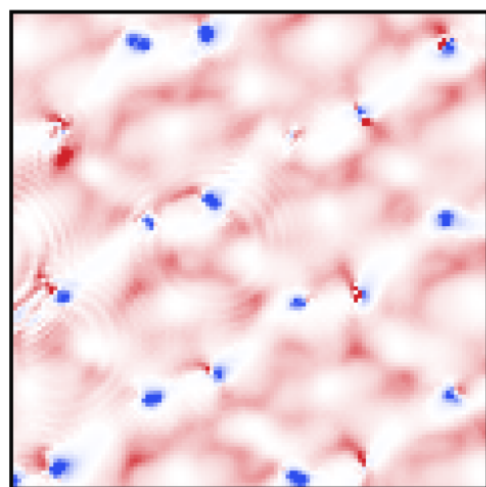

Supplement: Supplementary file 1 [file experiments_supplemental.pdf]
